# Supplementary material for: Gradient-Free Generation for Hard-Constrained Systems
Source: arXiv:2412.01786 source file (2025-03-03)
Supplement: Supplementary file 1 [file F_impact.tex]

\section{Broader Impact}
